# Supplementary material for: Hyperbolic vs Euclidean Embeddings in Few-Shot Learning: Two Sides of the Same Coin
Source: arXiv:2309.10013 source file (2023-09-18)
Supplement: Supplementary file 1 [file supp.tex]

\onecolumn
\begin{center}
\LARGE{\bf Hyperbolic vs Euclidean Embeddings in Few-Shot Learning: \\ Two Sides of the Same Coin \\ \large Supplementary Material }
\end{center}

\section{The hyperboloid model}
Consider the upper-sheet of a $d$-dimensional hyperboloid $H_k^d \subset \mathbb{R}^{d,1}$ as defined in (\ref{eq:definition_hyperboloid}). At each of its points $\mathbf{x} \in H^d_k$, we  have the tangent space as $T_{\mathbf{x}} H^d_k = \{\mathbf{v}\in \mathbb{R}^{d,1} : \langle \mathbf{x},\mathbf{v}\rangle_L =0\}$. For $\mathbf{v} \in T_{\mathbf{x}} H^d_k$, there is a unique geodesic $\gamma_{\mathbf{v}}: \mathbb{R} \to H^d_k$ such that $\gamma_{\mathbf{v}}'(0)=\mathbf{v}$. The exponential map $\mathrm{Exp}^H : T H^d_k\to H^d_k$ is defined as $\mathrm{Exp}^H_{\mathbf{x}}(\mathbf{v}) := \gamma_{\mathbf{v}}(1)$,
\begin{align}
    &\mathrm{Exp}_x^H(\mathbf{v}) := \gamma_{\mathbf{v}}(1) =\cosh\big(\| \mathbf{v} \|_L \sqrt{-k}\big)\mathbf{x} + \frac{\sinh\big(\|\mathbf{v}\|_L \sqrt{-k}\big)\mathbf{v}}{ \|\mathbf{v}\|_L \sqrt{-k}},
    \label{eq:hyperboloid_exp_map}
\end{align}
where $\|\mathbf{v}\|_L = \sqrt{\langle \mathbf{v}, \mathbf{v}\rangle_L}$, with $\langle\cdot,\cdot\rangle_L$ the Lorentz pseudometric (\ref{eq:lorentz_pseudometric}). Given two points $\mathbf{x},\mathbf{y} \in H^d_k$, the hyperbolic distance $d_{H^d_k}(\mathbf{x},\mathbf{y})$ is obtained by integrating the velocity of the geodesic between them,
\begin{equation}
    d_{H^d_k}(\mathbf{x},\mathbf{y}) := \frac{1}{\sqrt{-k}}\mathrm{acosh}(k \langle \mathbf{x},\mathbf{y} \rangle_L).
    \label{eq:hyperboloid_distance}
\end{equation}
We can verify that the hyperboloid $H_k^d$ and the Poincaré ball $P_k^d$ are isometric models of $d$-dimensional hyperbolic space with curvature $k$ \ie, for $\mathbf{x},\mathbf{y}\in H_k^d$
\begin{equation}
    d_{H_k^d}(\mathbf{x},\mathbf{y}) = d_{P_k^d}\left(\Pi(\mathbf{x}),\Pi(\mathbf{y})\right),
    \label{eq:hyperboloid_poincare_isometric}
\end{equation}
where $\Pi$ is the stereographic projection defined in (\ref{eq:stereographic_projection}). A comparison of geometries with constant positive, zero and negative curvature is presented in Table \ref{tab:geometries_comparison}. Note that $\langle\cdot,\cdot\rangle_E$ denotes the Euclidean inner product (dot product).

\begin{table}[h]
\begin{center}
\begin{tabular}{l|cc}
\toprule
Manifold & Curvature  & Geodesic $d(\mathbf{x},\mathbf{y})$\\
\midrule
    Euclidean $\mathbb{R}^d$  & $k=0$ & $\sqrt{\langle \mathbf{x}-\mathbf{y},\mathbf{x}-\mathbf{y}\rangle_E}$ \\
    Spherical $S_k^{d}\subset \mathbb{R}^{d+1}$ & $k > 0$  & $\frac{1}{\sqrt{k}}\mathrm{acos}(k \langle \mathbf{x},\mathbf{y}\rangle_E)$ \\
    Hyperbolic $H_k^d \subset \mathbb{R}^{d,1}$ & $k < 0$ & $\frac{1}{\sqrt{-k}}\mathrm{acosh}(k \langle\mathbf{x},\mathbf{y}\rangle_L)$ \\
\bottomrule
\end{tabular}
\end{center}
  \caption{Overview of the different isotropic geometries.}
  \label{tab:geometries_comparison}
\end{table}

\paragraph{Hyperbolic distance for fixed-radius embeddings}
Consider $\mathbf{x}$ and $\mathbf{y}$ in $P_k^d$ such that $\|\mathbf{x}\|_2 = \|\mathbf{y}\|_2 = r$ and $\angle(\mathbf{x},\mathbf{y}) = \alpha$. The hyperbolic distance between $\mathbf{x}$ and $\mathbf{y}$ can be computed using (\ref{eq:hyperboloid_poincare_isometric}). Recall that $\lambda(\mathbf{u})=2/(1+k\|\mathbf{u}\|_2^2)$. We have then
\begin{align}
    \left\langle\Pi^{-1}(\mathbf{x}),\Pi^{-1}(\mathbf{y})\right\rangle_L &= \lambda(\mathbf{x})\lambda(\mathbf{y})\left\langle\mathbf{x},\mathbf{y}\right\rangle_E + \frac{1}{k}(\lambda(\mathbf{x})-1)(\lambda(\mathbf{y})-1) \nonumber \\
    &= \frac{4}{(1+kr^2)^2}r^2\cos(\alpha) + \frac{1}{k}\left(\frac{1-kr^2}{1+kr^2}\right)^2.
\end{align}
Plugging this in (\ref{eq:hyperboloid_distance}) yields expression (\ref{eq:angular_poincare_dist}),
\begin{align}
    d_{P^d_k}(\mathbf{x},\mathbf{y}) = d_{H_k^d}(\Pi^{-1}(\mathbf{x}),\Pi^{-1}(\mathbf{y})) = \frac{1}{\sqrt{-k}}\mathrm{acosh}\left(\frac{4kr^2}{(1+kr^2)^2}\cos(\alpha) + \left(\frac{1-kr^2}{1+kr^2}\right)^2\right).
\end{align}

\section{Models}
\paragraph{Backbone} Similarly to \cite{Khrulkov2019HyperbolicEmbeddings}, the convolutional backbone used in all experiments consists of a sequence of 4 convolutional blocks, each of which composed of $3\times 3$ 2D Convolutions with 64 filters and stride 1, 2D Batch Normalization, ReLU activation and 2D MaxPool. The 4th block has as many filters as dimensions in the output manifold.

\paragraph{Scheduler} A StepLR scheduler was used to train all models. In the CUB dataset, the initial learning rate of $10^{-3}$ is decayed by a factor of $0.8$ every 40 epochs both in the 1s5w and the 5s5w few-shot settings. In the MiniImageNet dataset, the initial learning rate of $5\times 10^{-3}$ is decayed by a factor of $0.5$ every 80 epochs in the 1s5w setting (trained as 1s30w), and by $0.5$ every 60 epochs in the 5s5w scenario (trained as 5s20w). 

\paragraph{Image transformations}  In the case of the CUB\_200\_2011, we crop the images according to the bounding boxes provided in the dataset before other image transformations. The data augmentations performed during training were: 1) Zero padding along the smallest dimension to produce a square image; 2) Random crop resized to $84\times 84 \times 3$; 3) Image jitter with 0.4 brightness, 0.4 contrast and 0.4 hue; 4) Random horizontal flip; 5) Normalization. At test time, the images were zero padded, resized to $84 \times 84$ and normalized.
